# Supplementary material for: Quantum Noise Theory of Exceptional Point Sensors
Source: arXiv:1805.12001 ancillary file (2019-01-25)
Supplement: Supplementary file 1 [file supplementary_material.pdf]

# Quantum Noise Theory of Exceptional Point Sensors: Supplementary information

Mengzhen Zhang,[1,2] William Sweeney,[1,2] Chia Wei Hsu,[1,2] Lan Yang,[3] A. D. Stone,[1,2] and Liang Jiang[1,2]

[1] *Departments of Applied Physics and Physics, Yale University, New Haven, CT 06520, USA*
[2] *Yale Quantum Institute, Yale University, New Haven, CT 06520, USA*
[3] *Department of Electrical and Systems Engineering, Washington University, St Louis, Missouri 63130, USA*

**Contents**

**S.I. Introduction** 1

**S.II. General formulation of coupled mode theory** 1
A. Example of dissipation of a single mode 1
B. Example of amplification of a single mode 2
C. Linear scattering process of a two-coupled-mode system 2

**S.III. Gaussian process: quantum aspect of bosonic linear scattering process** 4

**S.IV. Precision limit of sensing** 5
A. Fisher information of Gaussian states measured by heterodyne detection 5
B. Quantum Fisher information of Gaussian states 6

**S.V. Exceptional point (EP) sensing** 6
A. Theory of EP sensing 6
B. Example of EP sensing with a parity-time symmetric system 7

**References** 8

## S.I. INTRODUCTION

In this supplementary material, we show detailed calculation and derivation of our key results based on coupled mode theory and Fisher information theory. This text is organized as follows: in Section S.II. we apply coupled mode theory to linear scattering bosonic processes which are crucial to our later derivation. In Section S.III, we discuss the transformation of Gaussian quantum states under linear bosonic processes. In Section S.IV., we introduce formulas for calculating Fisher information and quantum Fisher information of Gaussian states, which are the mathematical tools that set the precision limit of sensing. Details of our general theory of exotic precision improvement in exceptional point sensing are discussed in Section S.V, along with the application of the general result to the two-coupled-mode example. Further discussion on its robustness against being below lasing threshold is provided in Section S.V.

## S.II. GENERAL FORMULATION OF COUPLED MODE THEORY

Throughout this text, our discussion only involves linear scattering processes of bosonic modes, which can be completely calculated by coupled mode theory and play a central role to our discussion later on. Therefore, we introduce our notations of coupled mode theory in this beginning section. We first briefly review how to model a single dissipative mode using input-output theory in Subsection S.II A. After that in Subsection S.II B, we introduce how to model a single amplified mode. Then generic linear scattering processes can be modeled by proper generalization of the two basic examples. An example of the generalization to a two-coupled-mode system with both attenuation and amplification is demonstrated in Subsection S.II C.

### A. Example of dissipation of a single mode

Let $a$ be the complex amplitude of a bounded bosonic mode that experiences dissipation with amplitude damping rate $\gamma$. Such dissipation can be modeled by fictitiously coupling the bounded mode $a$ to some incoming (outgoing) channel, whose complex amplitude is $B_{\mathrm{in(out)}}$ . Then the dynamics of the system can be described by the *equation of motion*

$$\frac{d}{dt}a = -i\omega_0 a - \frac{\gamma}{2}a + \sqrt{\gamma}B_{\mathrm{in}}, \tag{S1}$$

and the *input-output relation*

$$B_{\mathrm{out}} = B_{\mathrm{in}} - \sqrt{\gamma}a, \tag{S2}$$

where the propagating channel $B_{\mathrm{in(out)}}$ dissipates the bounded mode with rate $\gamma$. Then the *Green's function* for mode $a$ is

$$\mathcal{G}(t) = \left(\frac{d}{dt} + i\omega_0 + \frac{\gamma}{2}\right)^{-1}, \tag{S3}$$

which can be transformed into frequency domain as

$$\mathcal{G}[\omega] = \left(i(\omega_0 - \omega) + \frac{\gamma}{2}\right)^{-1}. \tag{S4}$$

Also transforming the equation of motion and input-output relation into frequency domain, we obtain

$$a[\omega] = \mathcal{G}[\omega]\sqrt{\gamma}B_{\mathrm{in}}[\omega], \tag{S5}$$

and

$$B_{\text{out}}\left[\omega\right]=\left(1-\sqrt{\gamma}\mathcal{G}\left[\omega\right]\sqrt{\gamma}\right)B_{\text{in}}\left[\omega\right]. \tag{S6}$$

Obviously, the above results should keep the same for the case where a non-dissipative mode is coupled to an incoming(outgoing) channel with rate $\gamma$. Assuming that we can directly control and measure the incoming and outgoing channels, then the scattering process can be described by the *scattering amplitude*

$$S\left[\omega\right]:=\left(1-\sqrt{\gamma}\mathcal{G}\left[\omega\right]\sqrt{\gamma}\right). \tag{S7}$$

### B. Example of amplification of a single mode

Now we consider the case of amplification of a single mode with gain rate $\gamma$. According to [S1], assuming fictitious incoming(outgoing) channel $B_{\text{in(out)}}$, the equations of motion are

$$\frac{d}{dt}a=-i\omega_0 a+\frac{\gamma}{2}a-\sqrt{\gamma}B_{\text{in}}^{\dagger}, \tag{S8}$$

$$\frac{d}{dt}a^{\dagger}=i\omega_0 a^{\dagger}+\frac{\gamma}{2}a^{\dagger}-\sqrt{\gamma}B_{\text{in}}, \tag{S9}$$

and the input-output relations are

$$B_{\text{out}}=B_{\text{in}}-\sqrt{\gamma}a^{\dagger}, \tag{S10}$$

$$B_{\text{out}}^{\dagger}=B_{\text{in}}^{\dagger}-\sqrt{\gamma}a, \tag{S11}$$

where $(\cdot)^{\dagger}$ represents the creation operator of the corresponding bosonic mode. Just as the example in the previous section, these equations can also describe the system of a non-amplified mode coupled to the incoming(outgoing) channel via two-mode-squeezing-like interaction $-i\sqrt{\gamma}B^{\dagger}a^{\dagger}+h.c.$

Now we introduce the quadratures [S6]

$$q\left[\omega\right]=a\left[\omega\right]+a^{\dagger}\left[-\omega\right],\ p\left[\omega\right]=-i\left(a\left[\omega\right]-a^{\dagger}\left[-\omega\right]\right),$$

$$Q'_{\text{in(out)}}\left[\omega\right]=B_{\text{in(out)}}\left[\omega\right]+B^{\dagger}_{\text{in(out)}}\left[-\omega\right],$$

and

$$P'_{\text{in(out)}}\left[\omega\right]=-i\left(B_{\text{in(out)}}\left[\omega\right]-B^{\dagger}_{\text{in(out)}}\left[-\omega\right]\right).$$

Then we can transform the equations of motion and input-output relations into the frequency domain and represent them in this quadrature basis, as follows

$$\omega p\left[\omega\right]=\omega_0 p\left[\omega\right]+\frac{\gamma}{2}q\left[\omega\right]-\sqrt{\gamma}Q'_{\text{in}}\left[\omega\right], \tag{S12}$$

$$-\omega q\left[\omega\right]=-\omega_0 q\left[\omega\right]+\frac{\gamma}{2}p\left[\omega\right]+\sqrt{\gamma}P'_{\text{in}}\left[\omega\right], \tag{S13}$$

$$Q'_{\text{out}}\left[\omega\right]=Q'_{\text{in}}\left[\omega\right]-\sqrt{\gamma}q\left[\omega\right], \tag{S14}$$

$$P'_{\text{out}}\left[\omega\right]=P'_{\text{in}}\left[\omega\right]+\sqrt{\gamma}p\left[\omega\right]. \tag{S15}$$

It follows from the equations of motion that

$$\begin{pmatrix}q\left[\omega\right]\\ p\left[\omega\right]\end{pmatrix}=\mathcal{G}\left[\omega\right]\mathbf{D}\begin{pmatrix}Q'_{\text{in}}\left[\omega\right]\\ P'_{\text{in}}\left[\omega\right]\end{pmatrix}, \tag{S16}$$

with

$$\mathbf{D}=\begin{pmatrix}-\sqrt{\gamma} & \\ & \sqrt{\gamma}\end{pmatrix}, \tag{S17}$$

where the frequency domain Green's function is a real matrix

$$\begin{aligned}\mathcal{G}\left[\omega\right] &= \left(\omega\mathbf{\Omega}-\begin{pmatrix}\omega_0 & \frac{\gamma}{2}\\ -\frac{\gamma}{2} & \omega_0\end{pmatrix}\mathbf{\Omega}\right)^{-1}\\ &= -\mathbf{\Omega}\left(\omega\mathbf{I}-\begin{pmatrix}\omega_0 & \frac{\gamma}{2}\\ -\frac{\gamma}{2} & \omega_0\end{pmatrix}\right)^{-1},\end{aligned} \tag{S18}$$

with

$$\mathbf{\Omega}=\begin{pmatrix} & 1\\ -1 & \end{pmatrix}. \tag{S19}$$

The input-output relations lead to

$$\begin{pmatrix}Q'_{\text{out}}\left[\omega\right]\\ P'_{\text{out}}\left[\omega\right]\end{pmatrix}=\left(\mathbf{I}-\mathbf{D}^T\mathcal{G}\left[\omega\right]\mathbf{D}\right)\begin{pmatrix}Q'_{\text{in}}\left[\omega\right]\\ P'_{\text{in}}\left[\omega\right]\end{pmatrix}. \tag{S20}$$

Now we can define

$$\mathbf{S}\left[\omega\right]=\mathbf{I}-\mathbf{D}^T\mathcal{G}\left[\omega\right]\mathbf{D}, \tag{S21}$$

as the *scattering matrix.* One can check $\mathbf{S}\left[\omega\right]$ is symplectic, i.e., $\mathbf{S}\left[\omega\right]^T\mathbf{\Omega}_1\mathbf{S}\left[\omega\right]=\mathbf{\Omega}$ [S2]. Moreover, we make the following comments to emphasize the similarity between Eq. (S21) and Eq. (S7): (1) The matrix $\mathbf{\Omega}$ in Eq. (S19) is squared to $-1$, which plays the role of the the imaginary unit $i$ in Eq. (S4). (2) The matrix $\mathbf{D}$ in Eq. (S17) is squared to $\gamma\mathbf{I}$, which plays the role of of $\sqrt{\gamma}$ in Eq. (S7).

### C. Linear scattering process of a two-coupled-mode system

In the previous subsections, we demonstrated how to model loss or gain by coupling with a dissipative or amplifying channel. Now we consider a two-coupled-mode-system example with one mode attenuated and the other amplified, and with degenerate frequencies, whose dynamics is described by the equation of motion

$$\begin{aligned}\frac{d}{dt}\begin{pmatrix}a_1\\ a_2\end{pmatrix} &= -i\begin{pmatrix}\omega_0-i\frac{\kappa+\eta_1}{2} & g\\ g & \omega_0-i\frac{\eta_2-\kappa}{2}\end{pmatrix}\begin{pmatrix}a_1\\ a_2\end{pmatrix}\\ &\quad+\begin{pmatrix}\sqrt{\kappa} & 0\\ 0 & \sqrt{\kappa}\end{pmatrix}\begin{pmatrix}A_{\text{in},1}\\ A_{\text{in},2}\end{pmatrix}\\ &\quad+\begin{pmatrix}\sqrt{\eta_1} & 0\\ 0 & -\sqrt{\eta_2}\end{pmatrix}\begin{pmatrix}B_{\text{in},1}\\ B^{*}_{\text{in},2}\end{pmatrix},\end{aligned} \tag{S22}$$

and the input-output relation

$$\begin{pmatrix} A_{\text{out},1} \\ A_{\text{out},2} \end{pmatrix} = \begin{pmatrix} A_{\text{in},1} \\ A_{\text{in},2} \end{pmatrix} - \begin{pmatrix} \sqrt{\kappa} & 0 \\ 0 & \sqrt{\kappa} \end{pmatrix} \begin{pmatrix} a_1 \\ a_2 \end{pmatrix}. \quad \text{(S23)}$$

The intrinsic loss $\eta_1$ and gain $\eta_2$ are introduced by coupling with fictitious channels $B_{\text{in},1}$ and $B_{\text{in},2}$ respectively, and thus assuming their amplitudes are zero. Each mode ($a_{1(2)}$) is also passively coupled additionally with one external channel ($A_{1(2)}$) both with coupling rate $\kappa$. We assume the $A$-channels can be directly controlled and measured, while the $B$-channels cannot. Correspondingly, we will say that the $A$-channels are *accessible*, and the $B$-channels are *inaccessible*.

In order to simplify the exhibition of math, we now introduce the following conventions

$$\mathbf{a} = \begin{pmatrix} a_1 \\ a_2 \end{pmatrix}, \ \mathbf{A}_{\text{in(out)}} = \begin{pmatrix} A_{\text{in(out)},1} \\ A_{\text{in(out)},1} \end{pmatrix}, \ \mathbf{B}_{\text{in}} = \begin{pmatrix} B_{\text{in},1} \\ B_{\text{in},2} \end{pmatrix},$$

and

$$\mathbf{H} = \begin{pmatrix} \omega_0 - i\frac{\kappa+\eta_1}{2} & g \\ g & \omega_0 - i\frac{\eta_2-\kappa}{2} \end{pmatrix},$$

$$\mathbf{K}_{\text{ex}} = \begin{pmatrix} \sqrt{\kappa} & \\ & \sqrt{\kappa} \end{pmatrix}, \ \mathbf{K}'_{\text{ex}} = \mathbf{0},$$

$$\mathbf{K}_{\text{i}} = \begin{pmatrix} \sqrt{\eta_1} & \\ & 0 \end{pmatrix}, \ \mathbf{K}'_{\text{i}} = \begin{pmatrix} 0 & \\ & -\sqrt{\eta_2} \end{pmatrix}.$$

Then we can rewrite the equation of motion as

$$\frac{d}{dt}\mathbf{a} = -i\mathbf{H}\mathbf{a} + \mathbf{K}_{\text{ex}}\mathbf{A}_{\text{in}} + \mathbf{K}_{\text{i}}\mathbf{B}_{\text{in}} + \mathbf{K}'_{\text{i}}\mathbf{B}^{\dagger}_{\text{in}}, \quad \text{(S24)}$$

and the input-output relation as

$$\mathbf{A}_{\text{out}} = \mathbf{A}_{\text{in}} - \mathbf{K}_{\text{ex}}\mathbf{a}. \quad \text{(S25)}$$

Last but not the least, the following convention will be adopted throughout this text

$$\begin{pmatrix} B^*_{\text{in},1} & B^*_{\text{in},2} \end{pmatrix} \neq \mathbf{B}^{\dagger}_{\text{in}} = \begin{pmatrix} B^{\dagger}_{\text{in},1} \\ B^{\dagger}_{\text{in},2} \end{pmatrix}. \quad \text{(S26)}$$

For compatibility with our later discussion, we define the vectors of quadrature operators for the bosonic modes and channels as

$$\mathbf{q}[\omega] = \mathbf{a}[\omega] + \mathbf{a}^{\dagger}[-\omega], \ \mathbf{p}[\omega] = -i\left(\mathbf{a}[\omega] - \mathbf{a}^{\dagger}[-\omega]\right),$$

$$\mathbf{Q}_{\text{in(out)}}[\omega] = \mathbf{A}_{\text{in(out)}}[\omega] + \mathbf{A}^{\dagger}_{\text{in(out)}}[-\omega],$$

$$\mathbf{P}_{\text{in(out)}}[\omega] = -i\left(\mathbf{A}_{\text{in(out)}}[\omega] - \mathbf{A}^{\dagger}_{\text{in(out)}}[-\omega]\right),$$

$$\mathbf{Q}'_{\text{in(out)}}[\omega] = \mathbf{B}_{\text{in(out)}}[\omega] + \mathbf{B}^{\dagger}_{\text{in(out)}}[-\omega],$$

and

$$\mathbf{P}'_{\text{in(out)}}[\omega] = -i\left(\mathbf{B}_{\text{in(out)}}[\omega] - \mathbf{B}^{\dagger}_{\text{in(out)}}[-\omega]\right).$$

In a similar way as what we did in the last subsection, we can obtain a real matrix as the frequency domain Green's function

$$\mathcal{G}[\omega] = -\mathbf{\Omega}(\omega\mathbf{I} - \mathbf{M})^{-1} \quad \text{(S27)}$$

where

$$\mathbf{M} = \begin{pmatrix} \Re[\mathbf{H}] & -\Im[\mathbf{H}] \\ \Im[\mathbf{H}] & \Re[\mathbf{H}] \end{pmatrix} = \begin{pmatrix} \omega_0 & g & \frac{\kappa+\eta_1}{2} & 0 \\ g & \omega_0 & 0 & -\frac{\eta_2-\kappa}{2} \\ -\frac{\kappa+\eta_1}{2} & 0 & \omega_0 & g \\ 0 & \frac{\eta_2-\kappa}{2} & g & \omega_0 \end{pmatrix} \quad \text{(S28)}$$

is the *effective Hamiltonian* in quadrature basis (ordered as $q_1, q_2, p_1, p_2$), and

$$\mathbf{\Omega} = \begin{pmatrix} & & 1 & \\ & & & 1 \\ -1 & & & \\ & -1 & & \end{pmatrix} \quad \text{(S29)}$$

plays the role of imaginary unit since $\mathbf{\Omega}^2 = -\mathbf{I}$. Then the scattering process can be completely described by a linear transformation of quadrature operators

$$\begin{pmatrix} \mathbf{Q}_{\text{out}}[\omega] \\ \mathbf{P}_{\text{out}}[\omega] \end{pmatrix} = \tilde{\mathbf{S}}[\omega] \begin{pmatrix} \mathbf{Q}_{\text{in}}[\omega] \\ \mathbf{P}_{\text{in}}[\omega] \end{pmatrix} + \mathbf{L}[\omega] \begin{pmatrix} \mathbf{Q}'_{\text{in}}[\omega] \\ \mathbf{Q}'_{\text{in}}[-\omega] \\ \mathbf{P}'_{\text{in}}[\omega] \\ \mathbf{P}'_{\text{in}}[-\omega] \end{pmatrix}. \quad \text{(S30)}$$

In the above equation, the scattering matrix

$$\tilde{\mathbf{S}}[\omega] = \mathbf{I} - \kappa\mathcal{G}[\omega], \quad \text{(S31)}$$

obtained from Eqs. (S24&S27) describes the transformation of quadrature amplitudes, and the matrix

$$\mathbf{L}[\omega] = \mathcal{G}[\omega]\mathbf{D}_{\text{i}} \quad \text{(S32)}$$

describes the addition of noise that will be explained more explicitly in later sections, where

$$\mathbf{D}_{\text{i}} = \begin{pmatrix} \sqrt{\eta_1} & 0 & & \\ 0 & -\sqrt{\eta_2} & & \\ & & \sqrt{\eta_1} & 0 \\ & & 0 & \sqrt{\eta_2} \end{pmatrix}. \quad \text{(S33)}$$

For convenience of our later discussion, we introduce the notations of *dimensionless Green's function as*

$$\mathbf{G}[\omega] = \kappa\mathcal{G}[\omega], \quad \text{(S34)}$$

and *ratio matrix* as

$$\mathbf{R} = \kappa^{-1}\mathbf{D}_{\mathrm{i}}. \tag{S35}$$

Then we obtain

$$\tilde{\mathbf{S}}[\omega] = \mathbf{I} - \mathbf{G}[\omega], \tag{S36}$$

and

$$\mathbf{L}[\omega] = -\mathbf{G}[\omega]\,\mathbf{R}. \tag{S37}$$

At last, we would like to make the following remarks that will be useful in rest of the text:

1. We can safely drop "$[\omega]$" without causing any confusion, when we are only interested in the properties of the coupled-mode system at some fixed frequency.

2. It is easy to derive a dimensionless Green's function and a ratio matrix for any linear-coupled multi-bosonic-mode system. Therefore, the above two matrix functions $\tilde{\mathbf{S}}[\omega]$ and $\mathbf{L}[\omega]$ can be used to describe generic bosonic linear scattering processes.

## S.III. GAUSSIAN PROCESS: QUANTUM ASPECT OF BOSONIC LINEAR SCATTERING PROCESS

We investigate the transformation of Gaussian quantum states [S2] under linear scattering processes in this section. The results derived here are crucial to our application of Fisher information to exceptional point sensing schemes. We will always assume the inputs are Gaussian states, which are the closest quantum analogy to classical signals.

A multi-mode Gaussian state can be completely determined by the expectation values and covariance matrix of its quadrature operators. Let $\mathbf{Q}$ and $\mathbf{P}$ be the quadrature operators (already defined in the previous section) for propagating bosonic modes of a certain frequency in the frequency domain. We define the vector

$$\mu = \begin{pmatrix} \langle \mathbf{Q} \rangle \\ \langle \mathbf{P} \rangle \end{pmatrix}, \tag{S38}$$

as the *expectation value*, and the matrix

$$\mathbf{V} = \frac{1}{2}\begin{pmatrix} \left\langle (\mathbf{Q}-\langle\mathbf{Q}\rangle)^T(\mathbf{Q}-\langle\mathbf{Q}\rangle)\right\rangle & \left\langle (\mathbf{Q}-\langle\mathbf{Q}\rangle)^T(\mathbf{P}-\langle\mathbf{P}\rangle)\right\rangle \\ \left\langle (\mathbf{P}-\langle\mathbf{P}\rangle)^T(\mathbf{Q}-\langle\mathbf{Q}\rangle)\right\rangle & \left\langle (\mathbf{P}-\langle\mathbf{P}\rangle)^T(\mathbf{P}-\langle\mathbf{P}\rangle)\right\rangle \end{pmatrix} \tag{S39}$$

as the *covariance matrix*, where $\langle\cdot\rangle$ means calculating the expectation value of the observable with respect to the given quantum state.

A nice property of linear scattering processes is: if the inputs are Gaussian states, then the outputs are also Gaussian states [S2]. Let $\mu_{\mathrm{in(out)}}$ be the expectation value and $\mathbf{V}_{\mathrm{in(out)}}$ be the covariance matrix of the Gaussian state inputs(outputs) in the *accessible* channels. Then by matching the left hand side of Eq.(S30) with the quadrature operators of the *accessible* channels and by definitions of the objects, we obtain

$$\mu_{\mathrm{out}} = \tilde{\mathbf{S}}\mu_{\mathrm{in}} = (\mathbf{I}-\mathbf{G})\,\mu_{\mathrm{in}}, \tag{S40}$$

and

$$\begin{aligned}\mathbf{V}_{\mathrm{out}} &= \tilde{\mathbf{S}}\mathbf{V}_{\mathrm{in}}\tilde{\mathbf{S}}^T + \mathbf{L}\mathbf{V}'_{\mathrm{in}}\mathbf{L}^T \\ &= (\mathbf{I}-\mathbf{G})\,\mathbf{V}_{\mathrm{in}}\left((\mathbf{I}-\mathbf{G})\right)^T + \mathbf{G}\mathbf{R}\mathbf{V}'_{\mathrm{in}}\mathbf{R}^T\mathbf{G}^T,\end{aligned} \tag{S41}$$

where $\mathbf{V}'_{\mathrm{in}}$ is the covariance matrix for the inputs in the *inaccessible* channels. Without loss of generality, we have assumed the expectation value of the inaccessible inputs is $\mathbf{0}$ and will keep this assumption for the rest of the text. It is also worth mentioning that all covariance matrices of Gaussian states should be positive definite, i.e., all the eigenvalues of a covariance matrix are greater than zero.

Now we suppose the Green's function is also dependent of a parameter $\theta$ in the form of $\mathbf{G} = \mathbf{G}_\theta = -\mathbf{\Omega}\left(\theta\mathbf{\Pi} - \mathbf{M}\right)^{-1}$ with real matrices $\mathbf{\Pi}$ and $\mathbf{M}$ are arbitrary real matrices. We can understand $\theta\mathbf{\Pi}-\mathbf{M}$ as the dimensionless effective Hamiltonian in quadrature basis. The $\theta$-dependence can be introduced as a perturbation to the unperturbed dimensionless effective Hamiltonian $\mathbf{M}$. Then we obtain the following equations

$$\mu_\theta = (\mathbf{I}-\mathbf{G}_\theta)\,\mu_{\mathrm{in}}, \tag{S42}$$

and

$$\mathbf{V}_\theta = (\mathbf{I}-\mathbf{G}_\theta)\,\mathbf{V}_{\mathrm{in}}\,(\mathbf{I}-\mathbf{G}_\theta)^T + \mathbf{G}_\theta\mathbf{R}\mathbf{V}'_{\mathrm{in}}\mathbf{R}^T\mathbf{G}_\theta^T, \tag{S43}$$

where we have dropped "out"s in the subscripts of the expectation value and covariance matrix.

*Example: A two-mode parity-time-symmetric system with perturbation near lasing threshold* The parity-time-symmetric system we will discuss here is the same as the one introduced in Subsection. S.II C along with the additional assumption

$$\Gamma = \frac{g}{\kappa} = \frac{\kappa+\eta_1}{2\kappa} = \frac{\eta_2-\kappa}{2\kappa}, \tag{S44}$$

which is at the lasing threshold. We add the uniform frequency shift $\epsilon$ as the perturbation to the system. We

also set $\omega_0$ to be zero by tuning the moving the origin of our frequency spectrum. Therefore,

$$\mathbf{G}_\theta \;=\; -\mathbf{\Omega}\left(\theta\mathbf{\Pi}-\mathbf{M}\right)^{-1} \tag{S45}$$

with $\theta := \epsilon/\kappa$, where

$$\mathbf{\Pi} = \mathbf{I}$$

and

$$\mathbf{M} = (-\Gamma)\begin{pmatrix} & 1 & 1 & \\ 1 & & & -1 \\ -1 & & & 1 \\ & 1 & 1 & \end{pmatrix}.$$

As an example, we can assume the covariance matrix of the input in the accessible channels is

$$\mathbf{V}_{\text{in}} = (2n_{\text{in}}+1)\,\mathbf{I}_{4\times4}, \tag{S46}$$

and the covariance matrix of the input in the inaccessible channels is

$$\mathbf{V}'_{\text{in}} = (2n'_{\text{in}}+1)\,\mathbf{I}_{8\times8}, \tag{S47}$$

where $\mathbf{I}_{4\times4}$ and $\mathbf{I}_{8\times8}$ are identity matrices of order four and eight respectively [S7], and $n_{\text{in}}$ and $n'_{\text{in}}$ represent the thermal excitation number in the input state and reservoir. Then the covariance matrix of the output in the accessible channels is

$$\begin{aligned}\mathbf{V}_\theta \;=&\; (2n_{\text{in}}+1)\left(\mathbf{I}-\mathbf{G}_\theta\right)\left(\mathbf{I}-\mathbf{G}_\theta\right)^T \\ &+ (2n'_{\text{in}}+1)\,\mathbf{G}_\theta\mathbf{R}\mathbf{R}^T\mathbf{G}_\theta^T,\end{aligned}$$

The second term corresponds to the noise imported from the reservoirs, i.e., the *added noise.*

## S.IV. PRECISION LIMIT OF SENSING

### A. Fisher information of Gaussian states measured by heterodyne detection

Outcomes of a physical measurement should obey the probability distribution determined by the quantum state of the measured object and the measurement scheme. Assuming that the measurement outcomes $\mathbf{x}$ (a real vector in generic cases) obey the probability distribution $p_\theta(\mathbf{x})$, where $\theta$ is a real parameter determined by the quantum state and the measurement scheme, then the probability of obtaining the measurement outcome $\mathbf{x}$ is $p_\theta(\mathbf{x})\,d\mathbf{x}$ (which is $p_\theta(\mathbf{x})$ when $\mathbf{x}$ is a discrete). Here is a simple example: Let $\theta$ be the mean position of a particle moving in the free space with wave function of a Gaussian wave packet. Then the outcome of a position measurement should obey the Gaussian distribution with mean value $\theta$, supposing that the measurement can be done instantaneously. Moreover, $\theta$ is also determined by the physical state of the particle because its mean position will vary with time.

Given an $N$-mode Gaussian state with expectation value $\mu$ and covariance matrix $\mathbf{V}$, an ideal heterodyne detection on all of the $N$-modes results in a Gaussian probability distribution

$$g(\mathbf{x}) = \frac{(2\pi)^{-N/2}}{\sqrt{\det(\mathbf{V}+\mathbf{I})}}\exp\left[-\frac{1}{2}(\mathbf{x}-\bar{\mathbf{x}})^T(\mathbf{V}+\mathbf{I})^{-1}(\mathbf{x}-\bar{\mathbf{x}})\right], \tag{S48}$$

with mean value $\bar{\mathbf{x}} = \mu$ and covariance matrix $\mathbf{\Sigma} = \mathbf{V}+\mathbf{I}$ [S2], where the measurement outcome $\mathbf{x}$ is a $2N$-dimensional real vector.

Now let the Gaussian state be the output of a linear scattering process perturbed by the parameter $\theta$. Our goal is to estimate this unknown parameter $\theta$ by performing (probably multi-round) heterodyne measurement on the output, and using the measurement outcome to infer the value of $\theta$. The $\bar{\mathbf{x}}$ and $\mathbf{V}$ are dependent on $\theta$ and can be denoted by $\bar{\mathbf{x}}_\theta$ and $\mathbf{V}_\theta$ respectively. Therefore we can also denote the probability distribution $g$ by $g_\theta$. Such an inference cannot give us the true value of $\theta$ but rather an estimate $\hat{\theta}$, and we will have a different $\hat{\theta}$ for each estimation. In fact, the estimation value $\hat{\theta}$ will obey a probability distribution. In our situation, the true value of $\theta$ will be equal to the mean value with respect to this probability distribution. In other words, if we perform $N$ rounds of measurement (each estimation process will only use the outcome of one round of measurement), we will have $N$ estimations. And the mean value of these estimations will approach the true value if we let $N\to\infty$. Therefore, we can calculate the deviation $\delta\theta = \sqrt{\langle(\hat{\theta}-\theta)^2\rangle}$ and use it to quantify the precision of our estimation. We can obtain the estimation from the measurement outcomes in different ways. However there exists a smallest achievable deviation that is given by the so-called *Fisher information*, by the Cramer–Rao bound [S3]

$$\delta\theta \geq \frac{1}{\sqrt{N}\sqrt{I(\theta)}}, \tag{S49}$$

where $N$ is the number of rounds of measurement (and we

use all $N$ outcomes to estimate the parameter and count it as a single round of estimation). For a single-round measurement, this is

$$\delta\theta \geq \frac{1}{\sqrt{I(\theta)}}. \tag{S50}$$

In the following, we will use this lower bound of a single-round measurement as the quantification of the *precision limit of sensing processes.*

For our purpose, we now study the Fisher information of a Gaussian probability distribution. For a general probability distribution $p_\theta(\mathbf{x})$, Fisher information is defined by [S3]

$$I(\theta) = \int \left(\frac{\partial p_\theta(\mathbf{x})}{\partial\theta}\right)^2 p_\theta(\mathbf{x})\, d\mathbf{x} \tag{S51}$$

Now let the probability distribution be the Gaussian distribution $g_\theta(\mathbf{x})$ with mean value $\bar{\mathbf{x}}_\theta$, and covariance matrix $\mathbf{\Sigma}_\theta$ as functions of parameter $\theta$, then the Fisher information is obtained by applying Eq. (S51) to Eq. (S48)

$$I(\theta) = \frac{1}{2}\mathrm{Tr}\left(\mathbf{\Sigma}_\theta^{-1}\frac{d\mathbf{\Sigma}_\theta}{d\theta}\mathbf{\Sigma}_\theta^{-1}\frac{d\mathbf{\Sigma}_\theta}{d\theta}\right) + \left(\frac{d\bar{\mathbf{x}}_\theta}{d\theta}\right)^T \mathbf{\Sigma}_\theta^{-1}\frac{d\bar{\mathbf{x}}_\theta}{d\theta}, \tag{S52}$$

where we define

$$I_0 = \frac{1}{2}\mathrm{Tr}\left(\mathbf{\Sigma}_\theta^{-1}\frac{d\mathbf{\Sigma}_\theta}{d\theta}\mathbf{\Sigma}_\theta^{-1}\frac{d\mathbf{\Sigma}_\theta}{d\theta}\right), \tag{S53}$$

and

$$I_1(\theta) = \left(\frac{d\bar{\mathbf{x}}_\theta}{d\theta}\right)^T \mathbf{\Sigma}_\theta^{-1}\frac{d\bar{\mathbf{x}}_\theta}{d\theta}. \tag{S54}$$

Then we only need the $\bar{\mathbf{x}}_\theta$ and $\mathbf{\Sigma}_\theta$ for each situation. For the ideal heterodyne detection performed on all the modes, we have

$$\bar{\mathbf{x}}_\theta = \mu_\theta, \tag{S55}$$

and

$$\mathbf{\Sigma}_\theta = \mathbf{V}_\theta + \mathbf{I}. \tag{S56}$$

At last, a nice property of Fisher information is that it is always achievable by maximum likelihood estimation method [S3]. Let $\{\mathbf{x}_i\}_{i=1}^N$ be the measurement outcomes of $N$ rounds of measurement, obeying some arbitrary probability distribution $p_\theta(\mathbf{x})$. If we estimate the parameter $\theta$ using the formula

$$\hat{\theta} = \underset{\theta}{\mathrm{argmax}} \prod_{i=1}^N p_\theta(\mathbf{x}_i), \tag{S57}$$

then its variance satisfies

$$(\delta\theta)^2 = \frac{1}{N} I(\theta)^{-1} + o\left(\frac{1}{N^2}\right), \tag{S58}$$

which achieves the Cramer–Rao bound asymptotically when $N \to \infty$.

### B. Quantum Fisher information of Gaussian states

In the previous subsection, we introduced Fisher information to quantify the precision limit of sensing processes. Fisher information is calculated for a fixed measurement scheme. Naturally, people will ask if there is an optimal measurement scheme that can provide maximum Fisher information. This question can be answered by calculating Quantum Fisher information, which is obtained by maximizing the Fisher information over the set of all physically possible measurement schemes.

Quantum Fisher information of Gaussian states depending on parameter $\theta$ can be calculated using the formula [S4, S5]

$$\mathcal{I}(\theta) = \frac{1}{2}\mathrm{tr}\left(\mathbf{\Phi}_\theta\frac{d\mathbf{V}_\theta}{d\theta}\right) + \left(\frac{d\mu_\theta}{d\theta}\right)^T \mathbf{V}_\theta^{-1}\left(\frac{d\mu_\theta}{d\theta}\right), \tag{S59}$$

where $\mu_\theta$, $\mathbf{V}_\theta$ are amplitude and covariance matrix (in quadrature basis) of the Gaussian state, and $\mathbf{\Phi}_\theta$ is implicitly determined by

$$\frac{d\mathbf{V}_\theta}{d\theta} = \mathbf{V}_\theta\mathbf{\Phi}_\theta\mathbf{V}_\theta - \mathbf{\Omega}\mathbf{\Phi}_\theta\mathbf{\Omega}^T, \tag{S60}$$

with $\mathbf{\Omega}$ the fundamental symplectic matrix, satisfying $\mathbf{\Omega}^2 = -\mathbf{I}$. For convenience, we denote

$$\mathcal{I}_0(\theta) := \frac{1}{2}\mathrm{tr}\left(\mathbf{\Phi}_\theta\frac{d\mathbf{V}_\theta}{d\theta}\right), \tag{S61}$$

$$\mathcal{I}_1(\theta) := \left(\frac{d\mu_\theta}{d\theta}\right)^T \mathbf{V}_\theta^{-1}\left(\frac{d\mu_\theta}{d\theta}\right). \tag{S62}$$

$\mathcal{I}_1(\theta)$ is of the same form as $I_1(\theta)$ defined in the previous subsection in the sense of replacing $\bar{\mathbf{x}}_\theta$ with $\mu_\theta$.

Since there is no simple explicit analytic form of $\mathbf{\Phi}_\theta$, it's hard to analyze its $\theta$ dependence, generally speaking. However, as mentioned in [S5], for cases where the Gaussian states are very noisy, we have the following approximation

$$\mathbf{\Phi}_\theta \approx \mathbf{V}_\theta^{-1}\left(\frac{d\mathbf{V}_\theta}{d\theta}\right)\mathbf{V}_\theta^{-1}. \tag{S63}$$

So

$$\mathcal{I}_0(\theta) \approx \frac{1}{2}\mathrm{tr}\left(\mathbf{V}_\theta^{-1}\left(\frac{d\mathbf{V}_\theta}{d\theta}\right)\mathbf{V}_\theta^{-1}\frac{d\mathbf{V}_\theta}{d\theta}\right). \tag{S64}$$

This form becomes $I_0(\theta)$ if we replace $\mathbf{V}_\theta$ with $\mathbf{\Sigma}_\theta$.

## S.V. EXCEPTIONAL POINT (EP) SENSING

### A. Theory of EP sensing

In this subsection, we calculate Fisher information and quantum Fisher information for a linear scattering process with Gaussian input state. The linear scattering process is determined by a system with EP structure. We

will demonstrate that the scaling of precision enhancement is determined by the order of the exceptional point, i.e., for process with large classical noise (e.g., thermal noise), $I, \mathcal{I} \sim \theta^{-2k}$, where $k$ is smaller than or equal to the order of the EP and $\theta$ is the parameter to be estimated. It should be noted that we always assume lasing threshold is satisfied during the whole derivation in this subsection. However, at the end of next subsection, we will show that the conclusion still holds approximately when the lasing threshold condition is not strictly satisfied.

Let the dimensionless Green's function be $\mathbf{G}_\theta = -\mathbf{\Omega}\left(\theta\mathbf{\Pi} - \mathbf{M}\right)^{-1}$. Without loss of generality, we assume $\mathbf{\Pi} = \mathbf{I}$ and $\mathbf{M} = \oplus_l \mathbf{J}_{m_l}(0)$, where $\mathbf{J}_{m_l}(0)$ is a $m_l \times m_l$ nilpotent Jordan block, or simply speaking, the system Hamiltonian $\mathbf{M}$ contains $l$ exceptional point structure, each of which is of size $m_l$. For example,

$$\mathbf{J}_3(0) = \begin{pmatrix} 0 & 1 & \\ & 0 & 1 \\ & & 0 \end{pmatrix}, \ \mathbf{J}_2(0) \oplus \mathbf{J}_2(0) = \begin{pmatrix} 0 & 1 & & \\ & 0 & & \\ & & 0 & 1 \\ & & & 0 \end{pmatrix}. \tag{S65}$$

Since $\mathbf{M}$ plays the role of effective Hamiltonian, the system is at the exceptional point. The following conclusions will hold whenever there exist invertible matrices $\mathbf{X}$ and $\mathbf{Y}$, such that $\mathbf{G}_\theta = \mathbf{X}\left(\theta\mathbf{\Pi} - \mathbf{M}\right)^{-1}\mathbf{Y}$ with $\mathbf{\Pi}$ and $\mathbf{M}$ as defined above.

Let the Laurent expansion of dimensionless Green's function $\mathbf{G}_\theta = -\mathbf{\Omega}\left(\theta\mathbf{\Pi} - \mathbf{M}\right)^{-1}$ start with $-\theta^{-k}\mathbf{\Omega}\mathbf{C}_0$, with integer $k > 0$ and a constant matrix $\mathbf{C}_0$. Then it follows that $k$ is equal to the largest $m_l$ in $\mathbf{M} = \oplus_l \mathbf{J}_{m_l}(0)$. Recalling Eq.(S43), we also have

$$\begin{aligned} & \mathbf{G}_\theta^{-1}\mathbf{V}_\theta\left(\mathbf{G}_\theta^T\right)^{-1} \\ = \ & \left(\theta\mathbf{\Pi} - \mathbf{M} + \mathbf{\Omega}\right)\left(\mathbf{\Omega}\mathbf{V}_{\rm in}\mathbf{\Omega}^T\right)\left(\theta\mathbf{\Pi} - \mathbf{M} + \mathbf{\Omega}\right)^T \\ & + \mathbf{R}\left(\mathbf{\Omega}\mathbf{V}'_{\rm in}\mathbf{\Omega}^T\right)\mathbf{R}^T \\ = \ & \mathbf{C}_1 + o(\theta), \end{aligned} \tag{S66}$$

$$\begin{aligned} & \mathbf{G}_\theta^{-1}\left(\mathbf{V}_\theta + \mathbf{I}\right)\left(\mathbf{G}_\theta^T\right)^{-1} \\ = \ & \left(\theta\mathbf{\Pi} - \mathbf{M} + \mathbf{\Omega}\right)\left(\mathbf{\Omega}\mathbf{V}_{\rm in}\mathbf{\Omega}^T\right)\left(\theta\mathbf{\Pi} - \mathbf{M} + \mathbf{\Omega}\right)^T \\ & + \mathbf{R}\mathbf{V}'_{\rm in}\mathbf{R}^T \\ & + \left(\theta\mathbf{\Pi} - \mathbf{M}\right)\left(\theta\mathbf{\Pi} - \mathbf{M}\right)^T \\ = \ & \mathbf{C}_1 + \mathbf{M}\mathbf{M}^T + o(\theta), \end{aligned} \tag{S67}$$

where

$$\mathbf{C}_1 = \left(\mathbf{I} + \mathbf{M}\mathbf{\Omega}\right)\mathbf{V}_{\rm in}\left(\mathbf{I} + \mathbf{M}\mathbf{\Omega}\right)^T + \mathbf{R}\mathbf{V}'_{\rm in}\mathbf{R}^T. \tag{S68}$$

It is easy to check $\mathbf{C}_1$ is positive definite. More intuitively, the above equations imply that

$$\mathbf{V}_\theta = \theta^{-2k}\mathbf{\Omega}\mathbf{C}_0\mathbf{C}_1\mathbf{C}_0^T\mathbf{\Omega}^T + \cdots. \tag{S69}$$

We also have

$$\begin{aligned} \frac{d\mu_\theta}{d\theta} &= \frac{d\left(\mathbf{I} - \mathbf{G}_\theta\right)}{d\theta}\mu_{\rm in} = -\frac{d\mathbf{G}_\theta}{d\theta}\mu_{\rm in} \\ &= \mathbf{G}_\theta\mathbf{\Pi}\mathbf{\Omega}\mathbf{G}_\theta\mu_{\rm in} = \mathbf{G}_\theta\mathbf{\Omega}\mathbf{G}_\theta\mu_{\rm in}. \end{aligned} \tag{S70}$$

Then we have

$$\mathcal{I}_1(\theta) = \mu_{\rm in}^T\mathbf{C}_0^T\mathbf{C}_1\mathbf{C}_0\mu_{\rm in}\theta^{-2k} + \cdots, \tag{S71}$$

and

$$I_1(\theta) = \mu_{\rm in}^T\mathbf{C}_0^T\left(\mathbf{C}_1 + \mathbf{M}\mathbf{M}^T\right)\mathbf{C}_0\mu_{\rm in}\theta^{-2k} + \cdots, \tag{S72}$$

where the term $\mathbf{M}\mathbf{M}^T$ comes from the added noise introduced by heterodyne measurement according to Eq. (S67). Obviously, there always exists a $\mu_{in}$ such that the leading Laurent expansion of $\mathcal{I}_1(\theta)$ and $I_1(\theta)$is proportional to $\theta^{-2k}$.

We can also verify that

$$I_0(\theta) = \frac{1}{2}\mathrm{Tr}\left(\mathbf{\Sigma}_\theta^{-1}\frac{d\mathbf{\Sigma}_\theta}{d\theta}\mathbf{\Sigma}_\theta^{-1}\frac{d\mathbf{\Sigma}_\theta}{d\theta}\right) = C_3\theta^{-2k} + \cdots, \tag{S73}$$

and for noisy Gaussian states

$$\mathcal{I}_0 = \frac{1}{2}\mathrm{tr}\left(\mathbf{V}_\theta^{-1}\left(\frac{d\mathbf{V}_\theta}{d\theta}\right)\mathbf{V}_\theta^{-1}\frac{d\mathbf{V}_\theta}{d\theta}\right) = C_4\theta^{-2k} + \cdots, \tag{S74}$$

with $C_3$ and $C_4$ positive real numbers. Then finally, we obtain for exceptional point sensing with heterodyne detection, the Fisher information

$$I(\theta) \sim \alpha\theta^{-2k} + \cdots, \tag{S75}$$

with $\alpha$ some positive real number. And this is the highest scaling one can achieve at least for noisy Gaussian states because the quantum Fisher information also has the same scaling,

$$\mathcal{I}(\theta) \sim \beta\theta^{-2k} + \cdots, \tag{S76}$$

with $\beta$ another positive real number.

## B. Example of EP sensing with a parity-time symmetric system

We now apply our theory of EP sensing to the example introduced in Section **S.III** with the assumption of lasing threshold assumption, and discuss the robustness and limit of this EP scheme. The parameter $\theta$ is coupled to the system as a linear perturbation to the Hamiltonian

$$\mathbf{H}_\theta = \mathbf{H} - \theta\kappa\mathbf{I}. \tag{S77}$$

It follows that

$$\mathbf{G}_\theta = \left(\Gamma\begin{pmatrix} -1 & & & 1 \\ & 1 & 1 & \\ & -1 & -1 & \\ -1 & & & 1 \end{pmatrix} - \theta\mathbf{\Omega}\right)^{-1} \tag{S78}$$

with $\Gamma = \gamma/\kappa \sim O(1)$, which can also be written as

$$\mathbf{G}_\theta = -\mathbf{\Omega}\mathbf{P}\left(\theta\mathbf{I} - \begin{pmatrix} 0 & 1 & & \\ & 0 & & \\ & & 0 & 1 \\ & & & 0 \end{pmatrix}\right)^{-1}\mathbf{P}^{-1} \tag{S79}$$

with

$$\mathbf{P} = \begin{pmatrix} 0 & 0 & -1 & 1 \\ -1 & -1 & 0 & 0 \\ 1 & 0 & 0 & 0 \\ 0 & 0 & -1 & 0 \end{pmatrix}. \tag{S80}$$

So the effective Hamiltonian consists of two $2\times2$ nilpotent Jordan blocks. And the largest scaling of $\mathbf{G}_\theta$ should be $\theta^{-2}$. We can also check this directly by calculating its inverse,

$$\mathbf{G}_\theta = \begin{pmatrix} -\frac{\Gamma}{\theta^2} & 0 & \frac{1}{\theta} & \frac{\Gamma}{\theta^2} \\ 0 & \frac{\Gamma}{\theta^2} & \frac{\Gamma}{\theta^2} & \frac{1}{\theta} \\ -\frac{1}{\theta} & -\frac{\Gamma}{\theta^2} & -\frac{\Gamma}{\theta^2} & 0 \\ -\frac{\Gamma}{\theta^2} & -\frac{1}{\theta} & 0 & \frac{\Gamma}{\theta^2} \end{pmatrix}. \tag{S81}$$

Finally, the (quantum) Fisher information will scale with $\theta$ as $\theta^{-2\times2} = \theta^{-4}$.We also find that

$$\mathbf{G}_\theta \sim -\theta^{-2}\mathbf{\Omega}\mathbf{C}_0 \tag{S82}$$

with

$$\mathbf{C}_0 = \Gamma \begin{pmatrix} 0 & -1 & -1 & 0 \\ -1 & 0 & 0 & 1 \\ 1 & 0 & 0 & -1 \\ 0 & -1 & -1 & 0 \end{pmatrix}. \tag{S83}$$

Because rank $(\mathbf{C}_0) = 2$, so there are only two orthogonal directions in the four-dimensional space of input quadratures that may not provide the enhancement. More rigorously, all solutions to $\mathbf{C}_0\mu_{\text{in}} = 0$ span a two-dimensional subspace. And according to Eq.(S71), this is the subspace that may not provide the enhancement.

So far, the lasing threshold condition is assumed in the above calculation. We now consider the situation where the system is at the state close to lasing threshold, with $\frac{\kappa-\eta_2}{2\kappa} = \Gamma - \delta$, $\frac{\kappa+\eta_1}{2\kappa} = \Gamma + \delta$, and $\delta/\Gamma \ll 1$. That is, each unperturbed mode has an additional dissipation rate $\delta\kappa$. Now we have

$$\begin{aligned} \mathbf{G}_\theta &= \left( \Gamma \begin{pmatrix} -1 & & & 1 \\ & 1 & 1 & \\ & -1 & -1 & \\ -1 & & & 1 \end{pmatrix} - \delta\mathbf{I} - \theta\mathbf{\Omega} \right)^{-1} \\ &\sim |\theta - i\delta|^{-2}, \end{aligned} \tag{S84}$$

and hence $\mathcal{I}(\theta) \sim |\theta - i\delta|^{-4}$. So the upper bound of the quantum Fisher information scales as $\delta^{-4} \sim \mathcal{I}(\theta = 0)$. Generally speaking, for system which is not at lasing threshold, the upper bound of quantum Fisher information is given by $\alpha \|\mathbf{G}_{\theta=0}\|^2$ with $\alpha \sim O(1)$, where we have used the *trace norm*

$$\|\mathbf{G}_{\theta=0}\| = \text{Tr}\sqrt{\mathbf{G}_{\theta=0}\mathbf{G}^T_{\theta=0}}.$$

---


[S1] C. Gardiner and P. Zoller, *Quantum noise: a handbook of Markovian and non-Markovian quantum stochastic methods with applications to quantum optics*, Vol. 56 (Springer Science & Business Media, 2004).

[S2] C. Weedbrook, S. Pirandola, R. García-Patrön, N. J. Cerf, T. C. Ralph, J. H. Shapiro, and S. Lloyd, Rev. Mod. Phys. **84**, 621 (2012).

[S3] S.-i. Amari, *Information geometry and its applications*, Applied Mathematical Sciences, Vol. 194 (Springer Japan, Tokyo, 2016).

[S4] A. Monras, arXiv:1303.3682 (2013).

[S5] Z. Jiang, Phys. Rev. A **89**, 032128 (2014).

[S6] It is worth to mention that $\hat{a}^\dagger[-\omega] = (\hat{a}[\omega])^\dagger$ is the actual creation operator of the corresponding bosonic mode in the frequency domain, for $\hat{a}(t) = \frac{1}{\sqrt{2\pi}}\int \hat{a}[\omega]e^{-i\omega t}dt$.

[S7] In our example, the frequency of the incoming(outgoing) channel will perfectly match the resonant frequency of the bounded modes, so $[-\omega]$ frequency components coalesce with $[+\omega]$ frequency components for accessible channels because they are passively coupled to the system. However they will remain apart for the inaccessible channels, which leads to an eighth-order covariance matrix.
